# Supplementary material for: Federated Layer-Wise Exchange for Cross-Client Money Laundering Pattern Detection
Source: arXiv:2605.06433 source file (2026-10-12)
Supplement: Supplementary file 1 [file appendix-exchange-algorithm.tex]

\section{Layer-Wise Exchange Algorithm}
\label{app:exchange-algorithm}

\begin{algorithm}[H]
\caption{Layer-Wise Exchange}
\label{alg:layer-wise-exchange}
\begin{algorithmic}[1]
\Require Extended subgraphs $\{G_c\}_{c=1}^{C}$,
shared parameters $\Theta$, depth $L$, and owned-node labels
$\{y_v\}_{v\in V}$

\vspace{0.1in}
\Statex \textbf{Forward exchange}

\ForAll{clients $c$ in parallel}
    \State $\mathbf{h}^{(0)}_{v,c}
    \gets \phi_{\theta^{\mathrm{emb}}}(\mathbf{x}_v)$,
    $\quad \forall v\in V_c^{\mathrm{own}}$
\EndFor
\State $\textsc{ExchangeLayer}(0)$
\Comment{broadcast owned representations to remote copies}

\For{$l=0,\ldots,L-1$}
    \ForAll{clients $c$ in parallel}
        \ForAll{$v\in V_c^{\mathrm{own}}$}
            \State compute $\mathbf{h}^{(l+1)}_{v,c}$ using
            \eqref{eq:local-message-passing}
        \EndFor
    \EndFor
    \If{$l+1<L$}
        \State $\textsc{ExchangeLayer}(l+1)$
    \EndIf
\EndFor

\vspace{0.1in}
\Statex \textbf{Backward exchange}
\ForAll{clients $c$ in parallel}
    \State $L_c
    \gets
    \sum_{v\in V_c^{\mathrm{own}}}
    \ell\!\left(\mathbf{h}^{(L)}_{v,c},y_v\right)$
    \State $\boldsymbol{\delta}^{(L)}_{v,c}
    \gets
    \dfrac{\partial
    \ell(\mathbf{h}^{(L)}_{v,c},y_v)}
    {\partial \mathbf{h}^{(L)}_{v,c}}$,
    $\quad \forall v\in V_c^{\mathrm{own}}$
\EndFor

\For{$l=L-1,\ldots,0$}
    \ForAll{clients $c$ in parallel}
        \State backpropagate with 
        adjoints $\{\boldsymbol{\delta}^{(l+1)}_{v,c}:
        v\in V_c^{\mathrm{own}}\}$
        \State accumulate   $g_c^{(l)}$
        \State form partial adjoints $\boldsymbol{\delta}_{u \leftarrow c}^{(l,\mathrm{part})}$ for all
        $u\in V_c^{\mathrm{own}}\cup V_c^{\mathrm{rem}}$
    \EndFor

    \State $\textsc{BackwardExchangeLayer}(l)$
    \State
    \[
        \boldsymbol{\delta}_{u,c'}^{(l)}
        \gets
        \boldsymbol{\delta}_{u \leftarrow c'}^{(l,\mathrm{part})}
        +
        \sum_{c:\,u\in V_c^{\mathrm{rem}}}
        \boldsymbol{\delta}_{u \leftarrow c}^{(l,\mathrm{part})}
    \]
\EndFor

\ForAll{clients $c$ in parallel}
    \State $g_c^{\mathrm{emb}}
    \gets
    \displaystyle
    \sum_{v\in V_c^{\mathrm{own}}}
    \left(
    \frac{\partial \mathbf{h}^{(0)}_{v,c}}
    {\partial\theta^{\mathrm{emb}}}
    \right)^{\!\top}
    \boldsymbol{\delta}_{v,c}^{(0)}$
\EndFor

\vspace{0.1in}
\State \Return
$\{\mathbf{h}^{(L)}_{v,c}:v\in V_c^{\mathrm{own}}\}$ and
$\{g_c^{\mathrm{emb}},g_c^{(0)},\ldots,g_c^{(L-1)}\}$
\end{algorithmic}
\end{algorithm}
