# Supplementary material for: Federated Layer-Wise Exchange for Cross-Client Money Laundering Pattern Detection
Source: arXiv:2605.06433 source file (2026-10-12)
Supplement: Supplementary file 2 [file appendix-training-methods.tex]

\section{Background on Training Methods}
\label{appendix:background-training-methods}

We consider a global graph $G=(V,E)$ distributed across $C$ clients. 
We use $G_c$ to denote the extended subgraph available to client $c$ for local training. 
Let $f_{\Theta}$ be a GNN with model parameters $\Theta$, and let $\mathcal{L}_c(\Theta;G_c)$ denote the loss evaluated on the training nodes owned by client $c$. 
Unless otherwise stated, the global objective is written as a weighted sum of client losses:
\begin{equation}
    \min_{\Theta} 
    \sum_{c=1}^{C} 
    \frac{K_c}{K}
    \mathcal{L}_c(\Theta;G_c),
    \qquad
    K=\sum_{c=1}^{C}K_c.
\end{equation}

Here, $K_c$ denotes the number of training samples owned by client $c$. 
The training methods below differ in whether they use the full graph or client-local graphs, and in how frequently they synchronize model parameters or node representations.


\paragraph{Centralized training.}
Centralized training assumes that the full graph $G$ and all training labels are available to a single learner. 
The GNN aggregates over complete neighborhoods $\mathcal{N}(v)$ for every node $v\in V$, and optimizes
\begin{equation}
    \min_{\Theta} \mathcal{L}_{\mathrm{cent}}(\Theta;G).
\end{equation}

At training step $t$, the model parameters are updated by
\begin{equation}
    \Theta^{(t+1)}
    \leftarrow
    \Theta^{(t)}
    -
    \eta
    \nabla_{\Theta}
    \mathcal{L}_{\mathrm{cent}}(\Theta^{(t)};G),
\end{equation}
where $\eta$ is the learning rate. 
Since centralized training performs message passing on the complete graph, it serves as the performance upper bound in our experiments.

% The model is trained on the full graph $G$ with parameters $\Theta$, aggregating over complete neighborhoods $\mathcal{N}(v)$ for all $v \in V$. 
% This serves as an upper bound on performance.

\paragraph{Fully local training.} 
Fully local training removes all communication between clients. 
Each client $c$ maintains its own model parameters $\Theta_c$ and trains only on its local subgraph $G_c$. 
The local objective is
\begin{equation}
    \min_{\Theta_c} \mathcal{L}_c(\Theta_c;G_c),
\end{equation}
and the local update at step $t$ is
\begin{equation}
    \Theta_c^{(t+1)}
    \leftarrow
    \Theta_c^{(t)}
    -
    \eta
    \nabla_{\Theta_c}
    \mathcal{L}_c(\Theta_c^{(t)};G_c).
\end{equation}

Because neither parameters nor embeddings are exchanged, the models $\{\Theta_c\}_{c=1}^{C}$ may diverge freely across clients. 
Moreover, each client performs message passing only with the information available in $G_c$, so cross-client subgraph patterns may become locally unobservable.


\paragraph{Federated averaging (FedAvg).} 
% Each client trains locally on $G_c$ for $E$ local epochs, then a central server aggregates parameters weighted by client dataset size:
% \begin{equation}
%   \label{eq:fedavg}
%   \Theta^{(t+1)} = \sum_{c=1}^{C} \frac{|V_c^{\mathrm{own}}|}{\sum_{c'}
%   |V_{c'}^{\mathrm{own}}|} \, \Theta_c^{(t)}.
% \end{equation}
FedAvg trains a shared global model through periodic parameter aggregation. 
At communication round $t$, the server broadcasts the current global model $\Theta^{(t)}$ to the selected clients. 
Each client initializes its local model with this global model and performs $E$ local training epochs on $G_c$:
\begin{equation}
    \Theta_c^{(t,e+1)}
    \leftarrow
    \Theta_c^{(t,e)}
    -
    \eta
    \nabla_{\Theta_c}
    \mathcal{L}_c(\Theta_c^{(t,e)};G_c),
    \quad
    e=0,\ldots,E-1.
\end{equation}

After local training, clients upload their updated parameters to the server, which computes a weighted aggregation:
\begin{equation}
    \Theta^{(t+1)}
    \leftarrow
    \sum_{c=1}^{C}
    \frac{K_c}{K}
    \Theta_c^{(t,E)}.
\end{equation}

FedAvg synchronizes parameters only once per communication round. 
Therefore, clients share the same parameters immediately after aggregation, but their parameters may drift apart during local training. 
In graph learning, this means FedAvg can improve statistical learning over fully local training, but it does not by itself restore the missing cross-client messages required to recover centralized message passing.


\paragraph{Federated proximal optimization (FedProx).}
FedProx follows the same communication protocol as FedAvg but augments each client's local objective with a proximal term that penalizes deviation from the global model received at the start of the round:
\begin{equation}
    \min_{\Theta_c}
    \mathcal{L}_c(\Theta_c;G_c)
    +
    \frac{\mu}{2}
    \left\lVert \Theta_c - \Theta^{(t)} \right\rVert^2,
\end{equation}
where $\mu \geq 0$ controls the strength of the regularization and $\Theta^{(t)}$ is the global model broadcast at the start of round $t$. The local update at epoch $e$ becomes
\begin{equation}
    \Theta_c^{(t,e+1)}
    \leftarrow
    \Theta_c^{(t,e)}
    -
    \eta
    \left(
    \nabla_{\Theta_c}\mathcal{L}_c(\Theta_c^{(t,e)};G_c)
    +
    \mu\left(\Theta_c^{(t,e)}-\Theta^{(t)}\right)
    \right),
\end{equation}
and clients are aggregated identically to FedAvg after $E$ local epochs. By bounding how far local parameters can drift from the global model within a round, FedProx limits client divergence under heterogeneous data without requiring the per-step synchronization of Sync-SGD.


\paragraph{Synchronous stochastic gradient descent (Sync-SGD).}
Sync-SGD synchronizes parameters after each mini-batch rather than after several local epochs. 
At step $t$, all clients train the same model $\Theta^{(t)}$. 
Each client samples a mini-batch $\mathcal{B}_c^{(t)}$ from its local graph and computes a local gradient:
\begin{equation}
    g_c^{(t)}
    =
    \nabla_{\Theta}
    \mathcal{L}_c(\Theta^{(t)};\mathcal{B}_c^{(t)}).
\end{equation}

The server aggregates these gradients using batch-size weights:
\begin{equation}
    g^{(t)}
    =
    \sum_{c=1}^{C}
    \frac{|\mathcal{B}_c^{(t)}|}
    {\sum_{c'=1}^{C}|\mathcal{B}_{c'}^{(t)}|}
    g_c^{(t)}.
\end{equation}

The global model is then updated as
\begin{equation}
    \Theta^{(t+1)}
    \leftarrow
    \Theta^{(t)}
    -
    \eta g^{(t)}.
\end{equation}

Because all clients receive the same updated parameters after each mini-batch, Sync-SGD maintains parameter equivalence throughout training at a much finer granularity than FedAvg.
% This makes Sync-SGD a baseline training method for studying whether cross-client embedding exchange can approximate centralized message passing when the model parameters are synchronized at fine granularity.
